# Supplementary material for: EmoDiffTalk:Emotion-aware Diffusion for Editable 3D Gaussian Talking Head
Source: arXiv:2512.05991 source file (2025-12-10)
Supplement: Supplementary file 1 [file X_suppl1.tex]

\clearpage
\setcounter{page}{1}
\maketitlesupplementary

\section{Rationale}
\label{sec:rationale}
Having the supplementary compiled together with the main paper means that:
\begin{itemize}
\item The supplementary can back-reference sections of the main paper, for example, we can refer to \cref{sec:intro};
\item The main paper can forward reference sub-sections within the supplementary explicitly (e.g. referring to a particular experiment); 
\item When submitted to arXiv, the supplementary will already included at the end of the paper.
\end{itemize}
To split the supplementary pages from the main paper, you can use \href{https://support.apple.com/en-ca/guide/preview/prvw11793/mac#:~:text=Delete%20a%20page%20from%20a,or%20choose%20Edit%20%3E%20Delete).}{Preview (on macOS)}, \href{https://www.adobe.com/acrobat/how-to/delete-pages-from-pdf.html#:~:text=Choose%20%E2%80%9CTools%E2%80%9D%20%3E%20%E2%80%9COrganize,or%20pages%20from%20the%20file.}{Adobe Acrobat} (on all OSs), as well as \href{https://superuser.com/questions/517986/is-it-possible-to-delete-some-pages-of-a-pdf-document}{command line tools}.

\subsection{Coder 4 Geometry Diffusion }
To incorporate the AU coder obtained in Section 3.1 into the modeling of temporal geometry, we propose employing a diffusion model. This model comprises two processes: the forward process follows a Markov chain $q(\bm{x}^n_t \mid \bm{x}^{n-1}_t)$ for $n \in \{1, \dots, N\}$ that gradually adds Gaussian noise to $\bm{x}^0_t$ according to a variance schedule. The original sequence was replaced by noise and ultimately transformed into a standard normal distribution $q(\bm{x}^N_t \mid \bm{x}^{0}_t)$. The reverse process is to reconstruct the original sequence from the distribution $q(\bm{x}^{n-1}_t \mid \bm{x}^{n}_t)$. Therefore, the purpose of the denoising network is to approximate this distribution, thereby predicting either noisy [] or clean sequence [] $\hat{\bm{x}}^0_t$. Following the approach adopted in prior work [], we focus solely on the latter prediction. This prediction method better integrates geometric loss, providing more precise constraints on facial motion---a point already thoroughly demonstrated in [].\\
\textbf{Transformer-Based Denoising Network.}
Broadly speaking, our Transformer-Based Denoising Network adopts a structure similar to the decoder in Diffposetalk[], also using Hubert-extracted audio features as one of its inputs and incorporating a windowing mechanism. Our decoder architecture can be observed in the appendix. Here, we primarily highlight our distinct design choices: First, we utilize AU coders $\bm{E}_0...\bm{E}_T$ extracted from audio features as one input to guide the denoising process, rather than style information extracted from 2D video. Second, we employ mesh point positions $\bm{P}$ as the initial template, with the network learning the offsets of all mesh points $\Delta \bm{P}_t$ no longer represents the 3DMM coefficients $\bm{\beta}$. Naturally, learning point offsets presents greater challenges than predicting a priori 3DMM coefficients. Therefore, we designed a series of losses to constrain facial structural changes and conducted ablation experiments comparing our approach with simpler GRU networks predicting point offsets without diffusion strategies. Results are shown in (Table []), demonstrating our strategy's superiority. In summary, our method aims to leverage the AU Coder as a prompt to guide the denoising process, enabling accurate prediction of point offsets in the mesh template. It achieves a fine-grained binding between each dimension of the AU Coder and point offsets---that is, it learns the relationship between the AU Coder and point offsets. The denoising network then outputs the clean sequence as:
\begin{equation}
\hat{\bm{x}}^0_{0:T} = D_{\theta}(\bm{x}^n_{0:T}, \bm{P}, \bm{E}_{0:T}, \bm{A}_{0:T}, n)
\end{equation}
\textbf{Losses.}
To ensure the generated facial motions are both geometrically accurate and temporally coherent, we design a loss function that consists of different components:
(1) We employed a simple vertex loss function[],Calculate the Euclidean distance between the actual point offset and the predicted offset.
\begin{equation}
\mathcal{L}_{\text{vertex}} = \frac{1}{T \cdot V} \sum_{t=1}^{T} \sum_{v=1}^{V} \| \bm{x}^0_t(v) - \hat{\bm{x}}^0_t(v) \|_2
\end{equation}
(2) The Velocity Consistency Loss[] ensures temporal smoothness of the generated model by matching the motion velocities between the generated and ground-truth sequences, helping to avoid sudden changes in movement and promoting more natural transitions between frames. Building on this, the Acceleration Consistency Loss[] further considers the acceleration of motion, enhancing the temporal coherence of the generated sequences and reducing jittering. Together, these losses contribute to smoother and more realistic motion dynamics in the generated output.\text{where } $\Delta\bm{x}^0_t(v) = \bm{x}^0_t(v) - \bm{x}^0_{t-1}(v)$
\begin{equation}
\mathcal{L}_{\text{vel}} = \frac{1}{TV} \sum_{t=1}^{T} \sum_{v=1}^{V} \| \Delta\bm{x}^0_t(v) - \Delta\hat{\bm{x}}^0_t(v) \|_2
\end{equation}
\begin{equation}
\mathcal{L}_{\text{acc}} = \frac{1}{(T-1)V} \sum_{t=2}^{T} \sum_{v=1}^{V} \| \Delta^2\bm{x}^0_t(v) - \Delta^2\hat{\bm{x}}^0_t(v) \|_2
\end{equation}
\begin{equation}
\mathcal{L}_{motion} = {L}_{\text{vel}}+{L}_{\text{acc}}
\end{equation}
(3) The Deformation Regularization employs a Laplacian smoothing term[] to ensure the smoothness of the mesh during deformation. 
\begin{equation}
\mathcal{L}_{\text{deform}} = \frac{1}{T \cdot V} \sum_{t=}^{T} \sum_{v=1}^{V} \| \Delta \bm{p}_t(v) \|_2 + \lambda_{\text{lap}} \cdot \mathcal{L}_{\text{laplacian}}
\end{equation}
(4) Lip Synchronization[] focuses on ensuring that the lip movements of the generated model accurately correspond to the ground-truth lip movements during speech. This loss measures the difference between the predicted lip vertex positions and the actual lip positions across specific frames where lip movements occur.
\begin{equation}
\mathcal{L}_{\text{lip}} = \frac{1}{T_{\text{lip}} \cdot V_{\text{lip}}} \sum_{t \in \mathcal{T}_{\text{lip}}} \sum_{v \in \mathcal{V}_{\text{lip}}} \| \bm{x}^0_t(v) - \hat{\bm{x}}^0_t(v) \|_2
\end{equation}
\begin{equation}
\mathcal{L}_{\text{total}} = \lambda_{\text{vertex}} \mathcal{L}_{\text{vertex}} + \lambda_{\text{motion}} \mathcal{L}_{\text{motion}} + \lambda_{\text{deform}} \mathcal{L}_{\text{deform}} + \lambda_{\text{lip}} \mathcal{L}_{\text{lip}}
\end{equation}

\textbf{Canonical Appearance via Triplane.}
In traditional 3DGS, 48 out of the 59 parameters in each Gaussian distribution are used for SH (3rd-order) to capture viewpoint-dependent color. Recently, methods using triplanes to store features and decoding color via MLP have demonstrated superiority over traditional representations [][]. For GS talking heads, the generation process typically involves minimal strong light changes, with variations primarily manifesting in facial muscle details. These details have been demonstrated to be effectively simulated by opacity variations. Therefore, storing the space-intensive SH is unnecessary. Moreover, establishing a connection between features and GS is crucial for applying AU coders to appearance. Previous SH approaches, designed for handling variations, struggle to establish such a connection with AU coder-like features, as our experiments( )clearly demonstrate.  

Each 3D Gaussian is represented by the 3D point position $\mu$ 
and covariance matrix $\Sigma$, and the density function is formulated as:
\begin{equation}
g(x) = e^{-\frac{1}{2}(x-\mu)^T\Sigma^{-1}(x-\mu)}
\end{equation}

As 3D Gaussians can be formulated as a 3D ellipsoid, the covariance matrix $\Sigma$ is further formulated as:
\begin{equation}
\Sigma = RSS^TR^T
\end{equation}
where $S$ is a scale and $R$ is a rotation matrix. The 3D Gaussians are differentiable and can be easily projected to 2D splats for rendering.

Different from the original 3DGS that uses spherical harmonics for appearance modeling, we employ a triplane representation combined with MLP decoding for color generation. Specifically, each 3D Gaussian point queries features from three orthogonal feature planes ($XY$, $XZ$, and $YZ$ planes) and decodes them through an MLP network to produce the final RGB color.

In the differentiable rendering phase, $g(x)$ is multiplied by an opacity $\alpha$, then splatted onto 2D planes and blended to constitute colors for each pixel. Different from the original 3DGS that uses spherical harmonics for appearance modeling, we employ a triplane representation to generate the initial RGB color for each Gaussian point during the canonical stage. Specifically, the color $c$ for each point is generated by:
\begin{equation}
c = \mathcal{M}(F_{xy}(x,y) \oplus F_{xz}(x,z) \oplus F_{yz}(y,z))
\end{equation}
where $\mathcal{M}$ is an MLP decoder and $F_{xy}$, $F_{xz}$, $F_{yz}$ are triplane feature maps.

Once the canonical Gaussians are established, we store the precomputed RGB color $c$ directly. During animation, the color remains static while only the opacity undergoes dynamic changes. This design ensures color consistency while allowing expressive motion variations.

In this way, the appearance of a static head can be represented as 3D Gaussians $G$:
\begin{equation}
G \leftarrow \{\mu, S, R, \alpha, c\}
\end{equation}
where $\leftarrow$ means $G$ is a set of parameterized points, each represented by a parameter set on the right of the arrow, and $c$ is the precomputed RGB color generated from the triplane representation.

In our approach, the canonical 3D Gaussians $G_0$ represent a static head avatar and are learned from multi-view images of a moment without speech, usually the first frame of a video clip. The canonical 3D Gaussians $G_0$ are denoted as:
\begin{equation}
G_0 \leftarrow \{\mu_0, S_0, R_0, \alpha_0, c_0\}
\end{equation}

\textbf{Dynamic Appearance Modeling}
As seen in Section 3.3, we now have the position changes of points on the mesh. It is evident that the GS points on the face are bound to each vertex of the mesh.When creating the appearance, we followed the approach used in Emotalk3D[], adding OTF points to non-facial areas such as clothing and hair. These GS points are defined during static appearance modeling, and their position changes are driven by GS points bound to the face. The details can be found in the appendix().

The Scale property of GS remains frozen during the animation process. Multiple studies on 3D talking heads[][] have demonstrated that altering Scale has no discernible effect on the dynamic appearance.The following primarily introduces Rot Net,Feature line with OPC Net, which play a dominant role in dynamic appearance.\\
\textbf{Rot Net 4 Gaussian Rotation}
The rotation parameters of GS are obtained through a three-layer MLP decoder. We refer to this three-layer MLP structure as the Rot Net. It reads the position of GS,AU coders and assigns a relative static rotational angle offset to GS:
\begin{equation}
R_t = \mathcal{N}_{\text{Rot}}(R_0, E_t,\mu_t)
\end{equation}
$\mu_t$ is the GS position for timestep t.\\
\textbf{Learnable Feature Line}
For changes in opacity, we designed a compact Feature Line whose initial purpose was to store implicit features regarding variations in flame expression coefficients. Here, we repurpose it to store fine-grained features of AU coder changes related to opacity. Specifically, we define a learnable feature tensor $\mathcal{F} \in \mathbb{R}^{K \times Q \times D}$ where $K=17$ represents the number of AUs, $Q$ denotes the number of facial Gaussian points, and $D=16$ is the feature dimension. Unlike previous works[ ] that rely on discrete emotion categories (e.g., 8 predefined expressions), our approach embraces a continuous AU-based representation: AU coder. This shift from discrete to continuous representation enables smooth interpolation between expressions and supports infinite expression combinations through linear AU blending.

The Feature Line is structured as $\mathcal{F} = \{\mathbf{f}_k^i \in \mathbb{R}^{16} \mid k \in [1,17], i \in [1,Q]\}$, where each $\mathbf{f}_k^i$ encodes the learned opacity pattern for the $i$-th Gaussian point under the $k$-th AU. These features are initialized with small random values and optimized end-to-end during training.

Given an AU coder $\mathbf{E}_t = [e_1, e_2, \ldots, e_{17}]^T \in [0,5]^{17}$ at timestep $t$, we aggregate features through weighted combination:
\begin{equation}
\mathbf{f}_t^i = \sum_{k=1}^{17} w_k \cdot \mathbf{f}_k^i, \quad w_k = \frac{e_k}{\sum_{j=1}^{17} e_j + \epsilon}
\end{equation}
where $w_k$ represents the normalized weight for the $k$-th AU and $\epsilon=10^{-6}$ prevents division by zero.\\
\textbf{OPC Net for Gaussian Opacity}
The OPC Net integrates the aggregated features with complementary information through a three-layer MLP decoder $\mathcal{N}_{\text{OPC}}$:
\begin{equation}
\Delta \alpha_t^i = \mathcal{N}_{\text{OPC}}(\mathbf{f}_t^i, \mathbf{E}_t,\mu_t )
\end{equation}

To ensure numerically stable opacity transitions, we perform modulation in logit space:
\begin{equation}
\alpha_t^i = \sigma(\text{logit}(\alpha_0^i) + \tanh(\Delta \alpha_t^i) \cdot 0.5)
\end{equation}
where $\alpha_0^i$ is the canonical opacity and $\sigma(\cdot)$ is the sigmoid function. The $\tanh(\cdot)$ activation constrains the offset to prevent opacity saturation.\\
\textbf{Motion-Opacity Correlation Constraint.}
We observe that opacity changes should be correlated with geometric deformations: regions with rapid position changes (e.g., mouth opening, jaw movement) typically exhibit larger opacity variations, while stable regions (e.g., forehead, nose bridge) should maintain relatively constant opacity. To enforce this physical prior, we introduce a motion-opacity correlation loss:
\begin{equation}
\mathcal{L}_{\text{opcmotion}} = \lambda_{\text{opcmotion}} \sum_{i=1}^{Q} \left( \|\Delta \mu_t^i\|_2 - \gamma \cdot |\Delta \alpha_t^i| \right)^2
\end{equation}
where $\Delta \mu_t^i = \mu_t^i - \mu_0^i$ is the position displacement from canonical space, $\Delta \alpha_t^i$ is the opacity change, $\gamma$ is a scaling factor that balances the magnitude between position and opacity changes, and $\lambda_{\text{motion}}=0.001$ controls the constraint strength. This loss encourages the network to learn that large geometric deformations should be accompanied by proportional opacity adjustments, while static regions maintain stable opacity values.

We apply additional regularization to prevent feature explosion and ensure temporal coherence:
\begin{equation}
\mathcal{L}_{\text{reg}} = \lambda_{\text{sparse}} \|\mathcal{F}\|_1 + \lambda_{\text{smooth}} \sum_{k=1}^{K-1} \|\mathbf{f}_k - \mathbf{f}_{k+1}\|_2^2
\end{equation}
where $\lambda_{\text{sparse}}=0.01$ encourages sparsity and $\lambda_{\text{smooth}}=0.001$ promotes smoothness across AU space.\\
\textbf{3DGS Rasterizer and Training.}
During training, as the Gaussian point cloud undergoes densification and pruning operations, the Feature Line adapts accordingly: cloned points duplicate their features, split points share parent features, and pruned points remove their features. This dynamic adaptation maintains consistency throughout training.

At timestep $t$, the dynamic 3D Gaussians $G_t$ are formulated by combining the canonical representation with learned deformations:
\begin{equation}
G_t \leftarrow \{\mu_t, S_0, R_t, \alpha_t, c_0\}
\end{equation}

The rendering process follows the standard 3DGS rasterization pipeline. For each pixel, we accumulate contributions from all Gaussians in front-to-back order:
\begin{equation}
C(\mathbf{pi}) = \sum_{i \in \mathcal{N}} c_i \alpha_t^i \prod_{j=1}^{i-1}(1-\alpha_t^j)
\end{equation}
where $C(\mathbf{pi})$ is the final pixel color, $\mathcal{N}$ is the set of Gaussians affecting pixel $\mathbf{pi}$, and the product term represents accumulated transparency.\\
\textbf{Training Objective.}
The overall training objective combines multiple loss terms to ensure high-quality reconstruction while maintaining physical plausibility:
\begin{equation}
\mathcal{L}_{\text{total}} = \mathcal{L}_{\text{recon}} + \mathcal{L}_{\text{reg}} + \mathcal{L}_{\text{opcmotion}} + \mathcal{L}_{\text{dist}}
\end{equation}

The reconstruction loss $\mathcal{L}_{\text{recon}}$ measures photometric quality:
\begin{equation}
\mathcal{L}_{\text{recon}} = (1-\lambda_{\text{ssim}}) \mathcal{L}_1 + \lambda_{\text{ssim}} \mathcal{L}_{\text{ssim}}
\end{equation}
where $\mathcal{L}_1 = \|I_{\text{render}} - I_{\text{gt}}\|_1$ is the L1 loss between rendered and ground truth images, $\mathcal{L}_{\text{ssim}} = 1 - \text{SSIM}(I_{\text{render}}, I_{\text{gt}})$ measures structural similarity, and $\lambda_{\text{ssim}}=0.2$ balances the two terms.

The distance regularization $\mathcal{L}_{\text{dist}}$ constrains facial point movements to prevent unrealistic deformations:
\begin{equation}
\mathcal{L}_{\text{dist}} = \lambda_{\text{move}} \sum_{i=1}^{Q} \min(\|\Delta\mu_t^i\|_2, \tau)
\end{equation}
where $\tau$ is a threshold for maximum allowed displacement and $\lambda_{\text{move}}=0.1$ controls the constraint strength. This loss prevents facial Gaussians from drifting too far from their canonical positions.

\subsection{Photorealistic Talking Head Generation}

\textbf{2D-Based Methods.}

% Early 2D approaches, such as MakeItTalk \cite{makeittalk} and Wav2Lip \cite{wav2lip}, prioritized accurate lip synchronization but often lacked the ability to model nuanced facial expressions and large head movements, leading to limited expressiveness and potential artifacts. Recent methods have incorporated emotional controls through reference images or latent codes. For instance, EAMM \cite{eamm} enabled one-shot emotional editing using an emotion-aware motion model. However, a fundamental limitation of these purely 2D image-synthesis approaches is their lack of explicit 3D geometric consistency, which can result in unrealistic deformations under novel viewpoints or significant pose changes 
% .

\textbf{3D-Based Methods.}

% 3D-based approaches inherently excel in geometric consistency and viewpoint invariance. These methods can be further divided into those based on explicit 3D models (e.g., 3D morphable models, 3DMM) and those leveraging implicit neural representations. Methods like FaceFormer \cite{faceformer} and MeshTalk \cite{meshtalk} used transformers to regress 3D facial meshes from audio, ensuring precise lip movements. With the rise of neural rendering, NeRF-based techniques such as AD-NeRF \cite{ad-nerf} and GeneFace \cite{geneface} achieved photorealistic free-view synthesis by modeling the scene as a continuous volumetric field 
% . It is crucial to note that although GeneFace and similar methods output 2D video frames, their core innovation and representation—relying on NeRF—are fundamentally 3D-aware 
% . More recently, 3D Gaussian splatting (3DGS) has emerged as an efficient alternative for explicit spatial representation; GaussianHead \cite{gaussianhead} and PortraitGaussian \cite{portraitgaussian} enabled real-time high-fidelity rendering. EmoTalk3D \cite{emotalk3d} extended 3DGS to emotional talking heads but relied on discrete emotion labels, limiting fine-grained control. For one-shot 3D talking portrait synthesis, Real3D-Portrait \cite{real3dportrait} introduced an image-to-plane model for 3D reconstruction from a single image and a unified audio/video-to-motion model, significantly enhancing generalization capability 
% .

\subsection{Emotion Control in Talking Heads}

% Emotional control has progressed from categorical labels to continuous, multimodal interfaces. Early works like EmoGen \cite{emogen} used GANs to generate expressions from basic emotion tags. EMOTE \cite{emote} worked on disentangling speech content and emotion for more natural animations. A key challenge in this area is the effective disentanglement of the complex information within an audio signal, which contains not only semantic content but also paralinguistic cues like speech style and emotion 
% . Recent methods have explored fine-grained controls via facial action units (AUs); for example, AU-Net \cite{au-net} regressed facial movements from AU labels, while TalkCLIP \cite{talkclip} aligned text descriptions with AU-based expressions. CAFE-TALK \cite{cafe-talk} introduced a diffusion-transformer framework with coarse- and fine-grained multimodal controls, using a two-stage pipeline to disentangle audio and AU conditions. Similarly, FG-EmoTalk \cite{fg-emotalk} enabled granular expression editing but faced challenges in temporal leakage. Beyond deterministic models, generative approaches like DiffPoseTalk \cite{diffposetalk} employed a diffusion model to generate stylistic 3D facial animations and head poses from speech and style references.

% %------------------------------------------------------------------------
